# Supplementary material for: SemGeo-Gen: Unsupervised Generation of Approximate Cross-Instance Semantic-Geometric Correspondences
Source: arXiv:2610.32663 source file (2026-12-01)
Supplement: Supplementary file 3 [file keypointnet_protocol.tex]

For each model pair, we consider only keypoints whose semantic identifier appears in both models.

PCK is normalized by the target object bounding-box diagonal.

We filtered outliers models from each catgory that werent aligned in pose. 
