# Supplementary material for: SemGeo-Gen: Unsupervised Generation of Approximate Cross-Instance Semantic-Geometric Correspondences
Source: arXiv:2610.32663 source file (2026-12-01)
Supplement: Supplementary file 4 [file smooth_table.tex]

\begin{table*}[t]
\centering
\setlength{\tabcolsep}{3pt}
\renewcommand{\arraystretch}{1.05}
\resizebox{\textwidth}{!}{%
\begin{tabular}{l|ccccccc|ccccccc|ccccccc|ccccccc}
\toprule
Category & \multicolumn{7}{c}{PCK@0.05} & \multicolumn{7}{c}{PCK@0.10} & \multicolumn{7}{c}{PCK@0.15} & \multicolumn{7}{c}{PCK@0.20} \\
\cmidrule(lr){2-8}\cmidrule(lr){9-15}\cmidrule(lr){16-22}\cmidrule(lr){23-29}
 & $\lambda{=}0.05$ & $\lambda{=}0.1$ & $\lambda{=}0.2$ & $\lambda{=}0.3$ & $\lambda{=}0.5$ & $\lambda{=}0.7$ & $\lambda{=}1$ & $\lambda{=}0.05$ & $\lambda{=}0.1$ & $\lambda{=}0.2$ & $\lambda{=}0.3$ & $\lambda{=}0.5$ & $\lambda{=}0.7$ & $\lambda{=}1$ & $\lambda{=}0.05$ & $\lambda{=}0.1$ & $\lambda{=}0.2$ & $\lambda{=}0.3$ & $\lambda{=}0.5$ & $\lambda{=}0.7$ & $\lambda{=}1$ & $\lambda{=}0.05$ & $\lambda{=}0.1$ & $\lambda{=}0.2$ & $\lambda{=}0.3$ & $\lambda{=}0.5$ & $\lambda{=}0.7$ & $\lambda{=}1$ \\
\midrule
airplane & \textbf{.74} & .73 & .72 & .71 & .69 & .68 & .68 & .91 & \textbf{.91} & .90 & .90 & .90 & .89 & .89 & .96 & \textbf{.97} & .96 & .96 & .96 & .96 & .96 & .98 & \textbf{.98} & .98 & .98 & .98 & .98 & .98 \\
bathtub & .70 & \textbf{.71} & .70 & .70 & .69 & .69 & .69 & .87 & .87 & \textbf{.88} & .87 & .87 & .87 & .87 & .95 & .95 & \textbf{.95} & .95 & .95 & .95 & .95 & .98 & .98 & \textbf{.98} & .98 & .98 & .98 & .98 \\
bed & \textbf{.74} & .72 & .71 & .71 & .71 & .70 & .70 & \textbf{.91} & .90 & .90 & .90 & .90 & .90 & .89 & \textbf{.94} & .94 & .93 & .94 & .94 & .93 & .93 & \textbf{.98} & .97 & .97 & .98 & .98 & .97 & .97 \\
bottle & .84 & \textbf{.85} & .84 & .84 & .83 & .82 & .81 & .97 & .97 & .97 & \textbf{.97} & .97 & .96 & .96 & .99 & .99 & .99 & \textbf{.99} & .99 & .99 & .99 & 1. & 1. & \textbf{1.} & 1. & 1. & .99 & .99 \\
cap & .78 & .78 & .79 & .80 & \textbf{.81} & .81 & .80 & .95 & .96 & .97 & .97 & .97 & \textbf{.97} & .97 & .99 & .99 & 1. & \textbf{1.} & 1. & 1. & 1. & 1. & \textbf{1.} & 1. & \textbf{1.} & \textbf{1.} & \textbf{1.} & \textbf{1.} \\
car & .76 & .77 & .78 & .78 & .79 & \textbf{.79} & .79 & .95 & .95 & .95 & .95 & .95 & .95 & \textbf{.95} & .99 & .99 & .99 & .99 & .99 & .99 & \textbf{.99} & 1. & 1. & 1. & 1. & 1. & 1. & \textbf{1.} \\
chair & \textbf{.80} & .78 & .75 & .74 & .71 & .70 & .68 & .96 & .96 & \textbf{.96} & .96 & .96 & .96 & .95 & .99 & .99 & \textbf{1.} & 1. & .99 & .99 & .99 & 1. & 1. & \textbf{1.} & \textbf{1.} & \textbf{1.} & \textbf{1.} & \textbf{1.} \\
guitar & \textbf{.80} & .80 & .79 & .79 & .78 & .77 & .76 & .95 & .95 & .95 & \textbf{.95} & .95 & .95 & .94 & .98 & .97 & .98 & .98 & .98 & \textbf{.98} & .98 & .99 & .99 & .99 & .99 & .99 & .99 & \textbf{.99} \\
helmet & .51 & .52 & .52 & .54 & .55 & .55 & \textbf{.56} & .78 & .77 & .78 & .79 & .80 & \textbf{.81} & .81 & .90 & .89 & .90 & .91 & .91 & .92 & \textbf{.92} & .95 & .95 & .95 & .95 & .95 & .95 & \textbf{.95} \\
knife & .78 & .78 & \textbf{.79} & .78 & .77 & .74 & .71 & \textbf{.88} & .88 & .88 & .87 & .87 & .86 & .86 & .93 & .93 & .94 & .94 & \textbf{.94} & .94 & .94 & .97 & .97 & \textbf{.97} & .97 & .96 & .96 & .96 \\
laptop & .90 & .90 & \textbf{.90} & .90 & .89 & .88 & .85 & .99 & .99 & \textbf{1.} & 1. & 1. & .99 & .99 & \textbf{1.} & \textbf{1.} & \textbf{1.} & \textbf{1.} & \textbf{1.} & \textbf{1.} & \textbf{1.} & \textbf{1.} & \textbf{1.} & \textbf{1.} & \textbf{1.} & \textbf{1.} & \textbf{1.} & \textbf{1.} \\
motorcycle & .75 & .75 & \textbf{.75} & .74 & .74 & .74 & .73 & .92 & .92 & \textbf{.92} & .92 & .92 & .92 & .92 & .98 & .98 & .98 & .98 & \textbf{.98} & .98 & .98 & 1. & 1. & 1. & \textbf{1.} & 1. & 1. & 1. \\
mug & .69 & .69 & .70 & \textbf{.71} & .70 & .69 & .68 & .95 & .95 & .96 & \textbf{.96} & .96 & .95 & .95 & .99 & .99 & \textbf{.99} & .99 & .99 & .99 & .99 & 1. & \textbf{1.} & 1. & 1. & 1. & 1. & 1. \\
skateboard & \textbf{.90} & .90 & .89 & .89 & .87 & .86 & .84 & .99 & \textbf{.99} & .98 & .98 & .98 & .98 & .98 & 1. & \textbf{1.} & 1. & 1. & 1. & 1. & 1. & \textbf{1.} & 1. & 1. & 1. & 1. & 1. & 1. \\
table & \textbf{.87} & .83 & .79 & .77 & .75 & .74 & .73 & \textbf{.98} & .98 & .97 & .96 & .94 & .93 & .92 & \textbf{1.} & 1. & .99 & .99 & .99 & .99 & .98 & \textbf{1.} & 1. & 1. & 1. & 1. & 1. & .99 \\
vessel & .51 & \textbf{.52} & .51 & .49 & .49 & .50 & .47 & .75 & \textbf{.76} & .75 & .74 & .74 & .74 & .72 & .89 & \textbf{.90} & .89 & .88 & .88 & .87 & .86 & \textbf{.97} & .97 & .97 & .97 & .97 & .97 & .96 \\
\midrule
Mean & \textbf{.75} & .75 & .75 & .74 & .74 & .73 & .72 & .92 & \textbf{.92} & .92 & .92 & .92 & .92 & .91 & .97 & .97 & \textbf{.97} & .97 & .97 & .97 & .97 & \textbf{.99} & .99 & .99 & .99 & .99 & .99 & .99 \\

\bottomrule
\end{tabular}%
}
\caption{Per-category PCK at thresholds $\{0.05, 0.10, 0.15, 0.20\}$ for varying smoothness weights $\lambda$. Best $\lambda$ per (category, threshold) in \textbf{bold}. Reporting results over 40 models per category.}
\label{tab:smooth_ablation}
\end{table*}
